# Supplementary material for: Learning to Explore Indoor Environments using Autonomous Micro Aerial Vehicles
Source: arXiv:2309.06986 source file (2023-09-13)
Supplement: Supplementary file 1 [file Appendix.tex]

\section{\\Action Space Definition}

Action space is shown in Table \ref{table:ac_space}.
\begin{table}[h!]
\begin{tabu}{|>{\centering}m{0.965cm} |>{\centering}m{.727cm} | >{\centering}m{.727cm} | >{\centering}m{.727cm} | >{\centering}m{.727cm} | >{\centering}m{.727cm} | >{\centering}m{.727cm} |} 
 \tabucline{-}
 \strut current action / previous action \strut & 0 & 1 & 2 & 3 & 4 & 5 \\
 \tabucline{-}
 \multirow{2}{0.965cm}{\centering 0} 
 & 0    & 0    & 0    & 0.075& 0.055& 0.055 \\
 & 0    &-0.1  & 0.1  & 0    &-0.1  & 0.1   \\
 \hline
 \multirow{2}{0.965cm}{\centering 1} 
 & 0    & 0    & 0    & 0.075& 0.055& 0.055 \\
 &-0.08 &-0.21 & 0.005&-0.08 &-0.21 & 0.005 \\
 \hline
 \multirow{2}{0.965cm}{\centering 2} 
 & 0    & 0    & 0    & 0.075& 0.055& 0.055 \\
 & 0.08 &-0.005& 0.21 & 0.08 &-0.005& 0.21  \\ 
 \hline
 \multirow{2}{0.965cm}{\centering 3} 
 & 0.17& 0.17  & 0.17 & 0.26 & 0.205& 0.205 \\
 & 0   &-0.1   & 0.1  & 0    &-0.1  & 0.1   \\ 
 \hline
 \multirow{2}{0.965cm}{\centering 4} 
 & 0.115& 0.115& 0.115& 0.22 & 0.18 & 0.15  \\
 &-0.08 &-0.21 & 0.005&-0.08 &-0.21 & 0.005 \\
 \hline 
 \multirow{2}{0.965cm}{\centering 5} 
 & 0.115& 0.115& 0.115& 0.22 & 0.18 & 0.15  \\
 & 0.08 &0.005 & 0.21 & 0.08 &-0.005& 0.21  \\ 
 \tabucline{-}
\end{tabu}

\caption{Action Space. In each cell the first element is the movement in meters and the second element is the rotation in radians \todo{TODO: better looking table.}}
\label{table:ac_space}
\end{table}
